# Supplementary material for: Towards Corruption-Agnostic Robust Domain Adaptation
Source: arXiv:2104.10376 source file (2021-04-21)
Supplement: Supplementary file 8 [file 15corruptions.tex]

\begin{figure*}[h]
    \centering
    \includegraphics[width=0.85\textwidth]{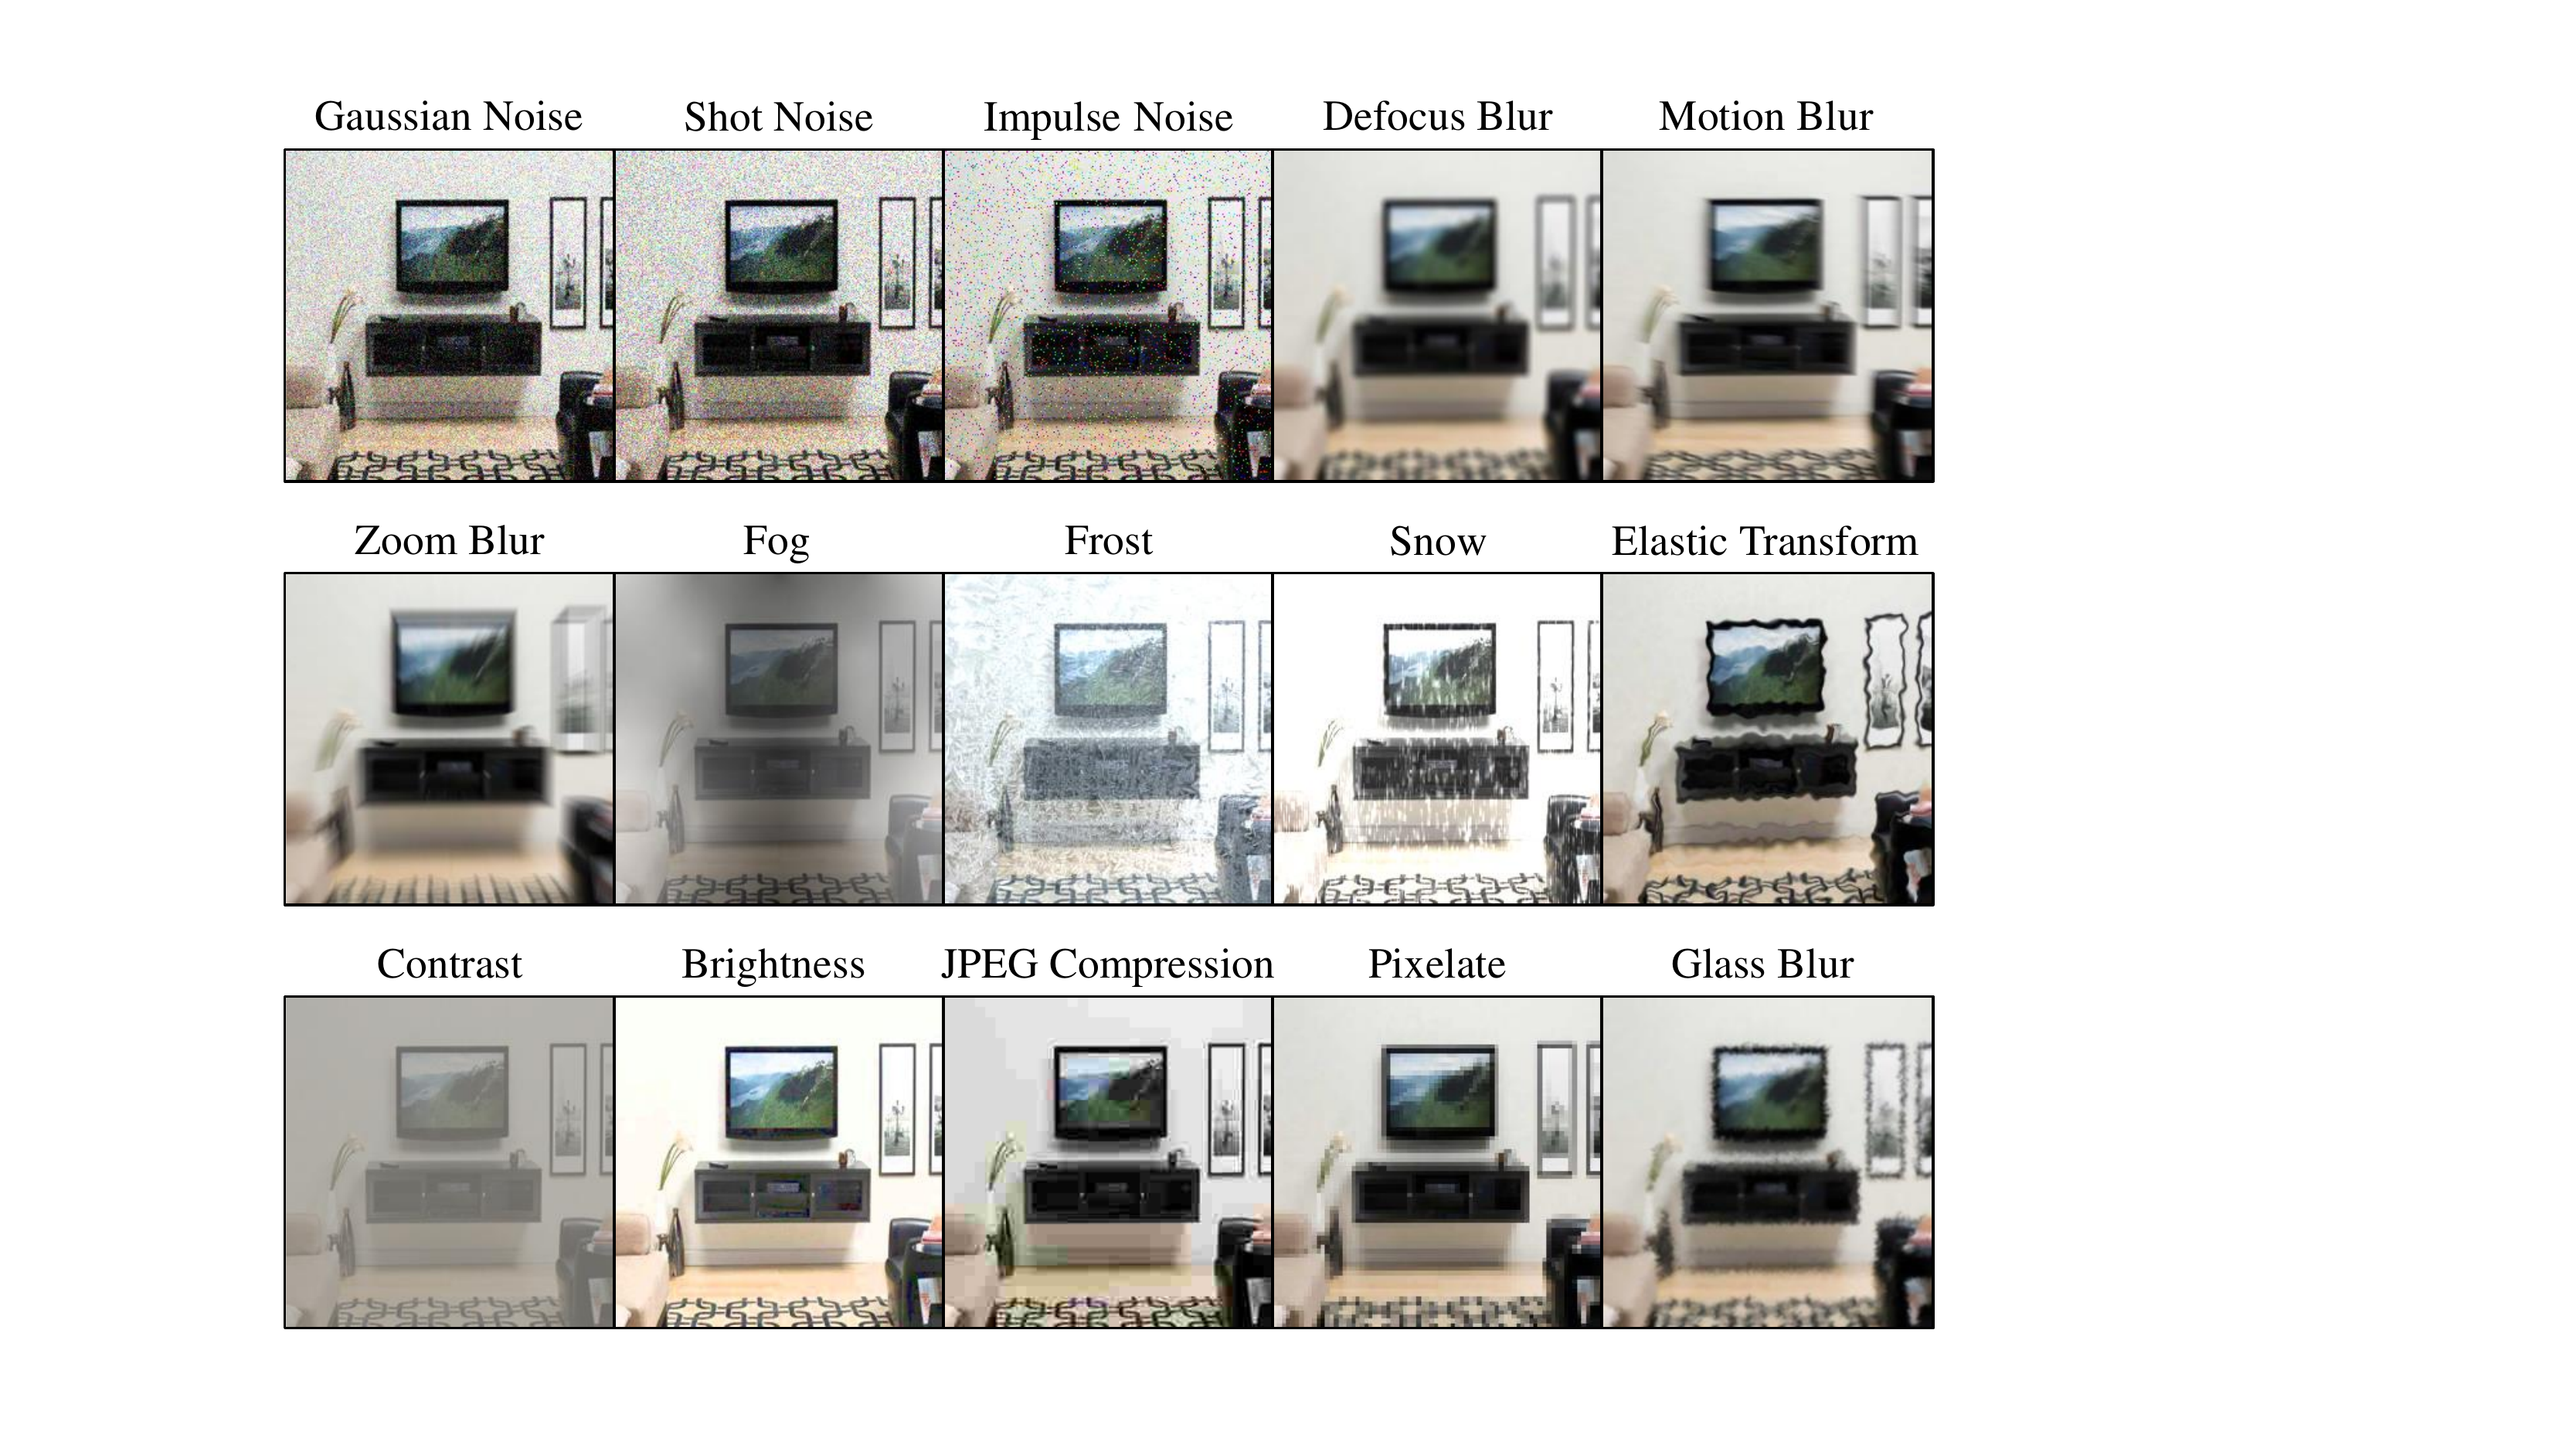}
    \caption{Examples of 15 kinds of corruptions.}
    \label{fig:15corruption}
\end{figure*}
