# Supplementary material for: Towards Corruption-Agnostic Robust Domain Adaptation
Source: arXiv:2104.10376 source file (2021-04-21)
Supplement: Supplementary file 10 [file mCE_office-sup.tex]

\begin{figure}[t]
    \centering
    \includegraphics[width=0.45\textwidth]{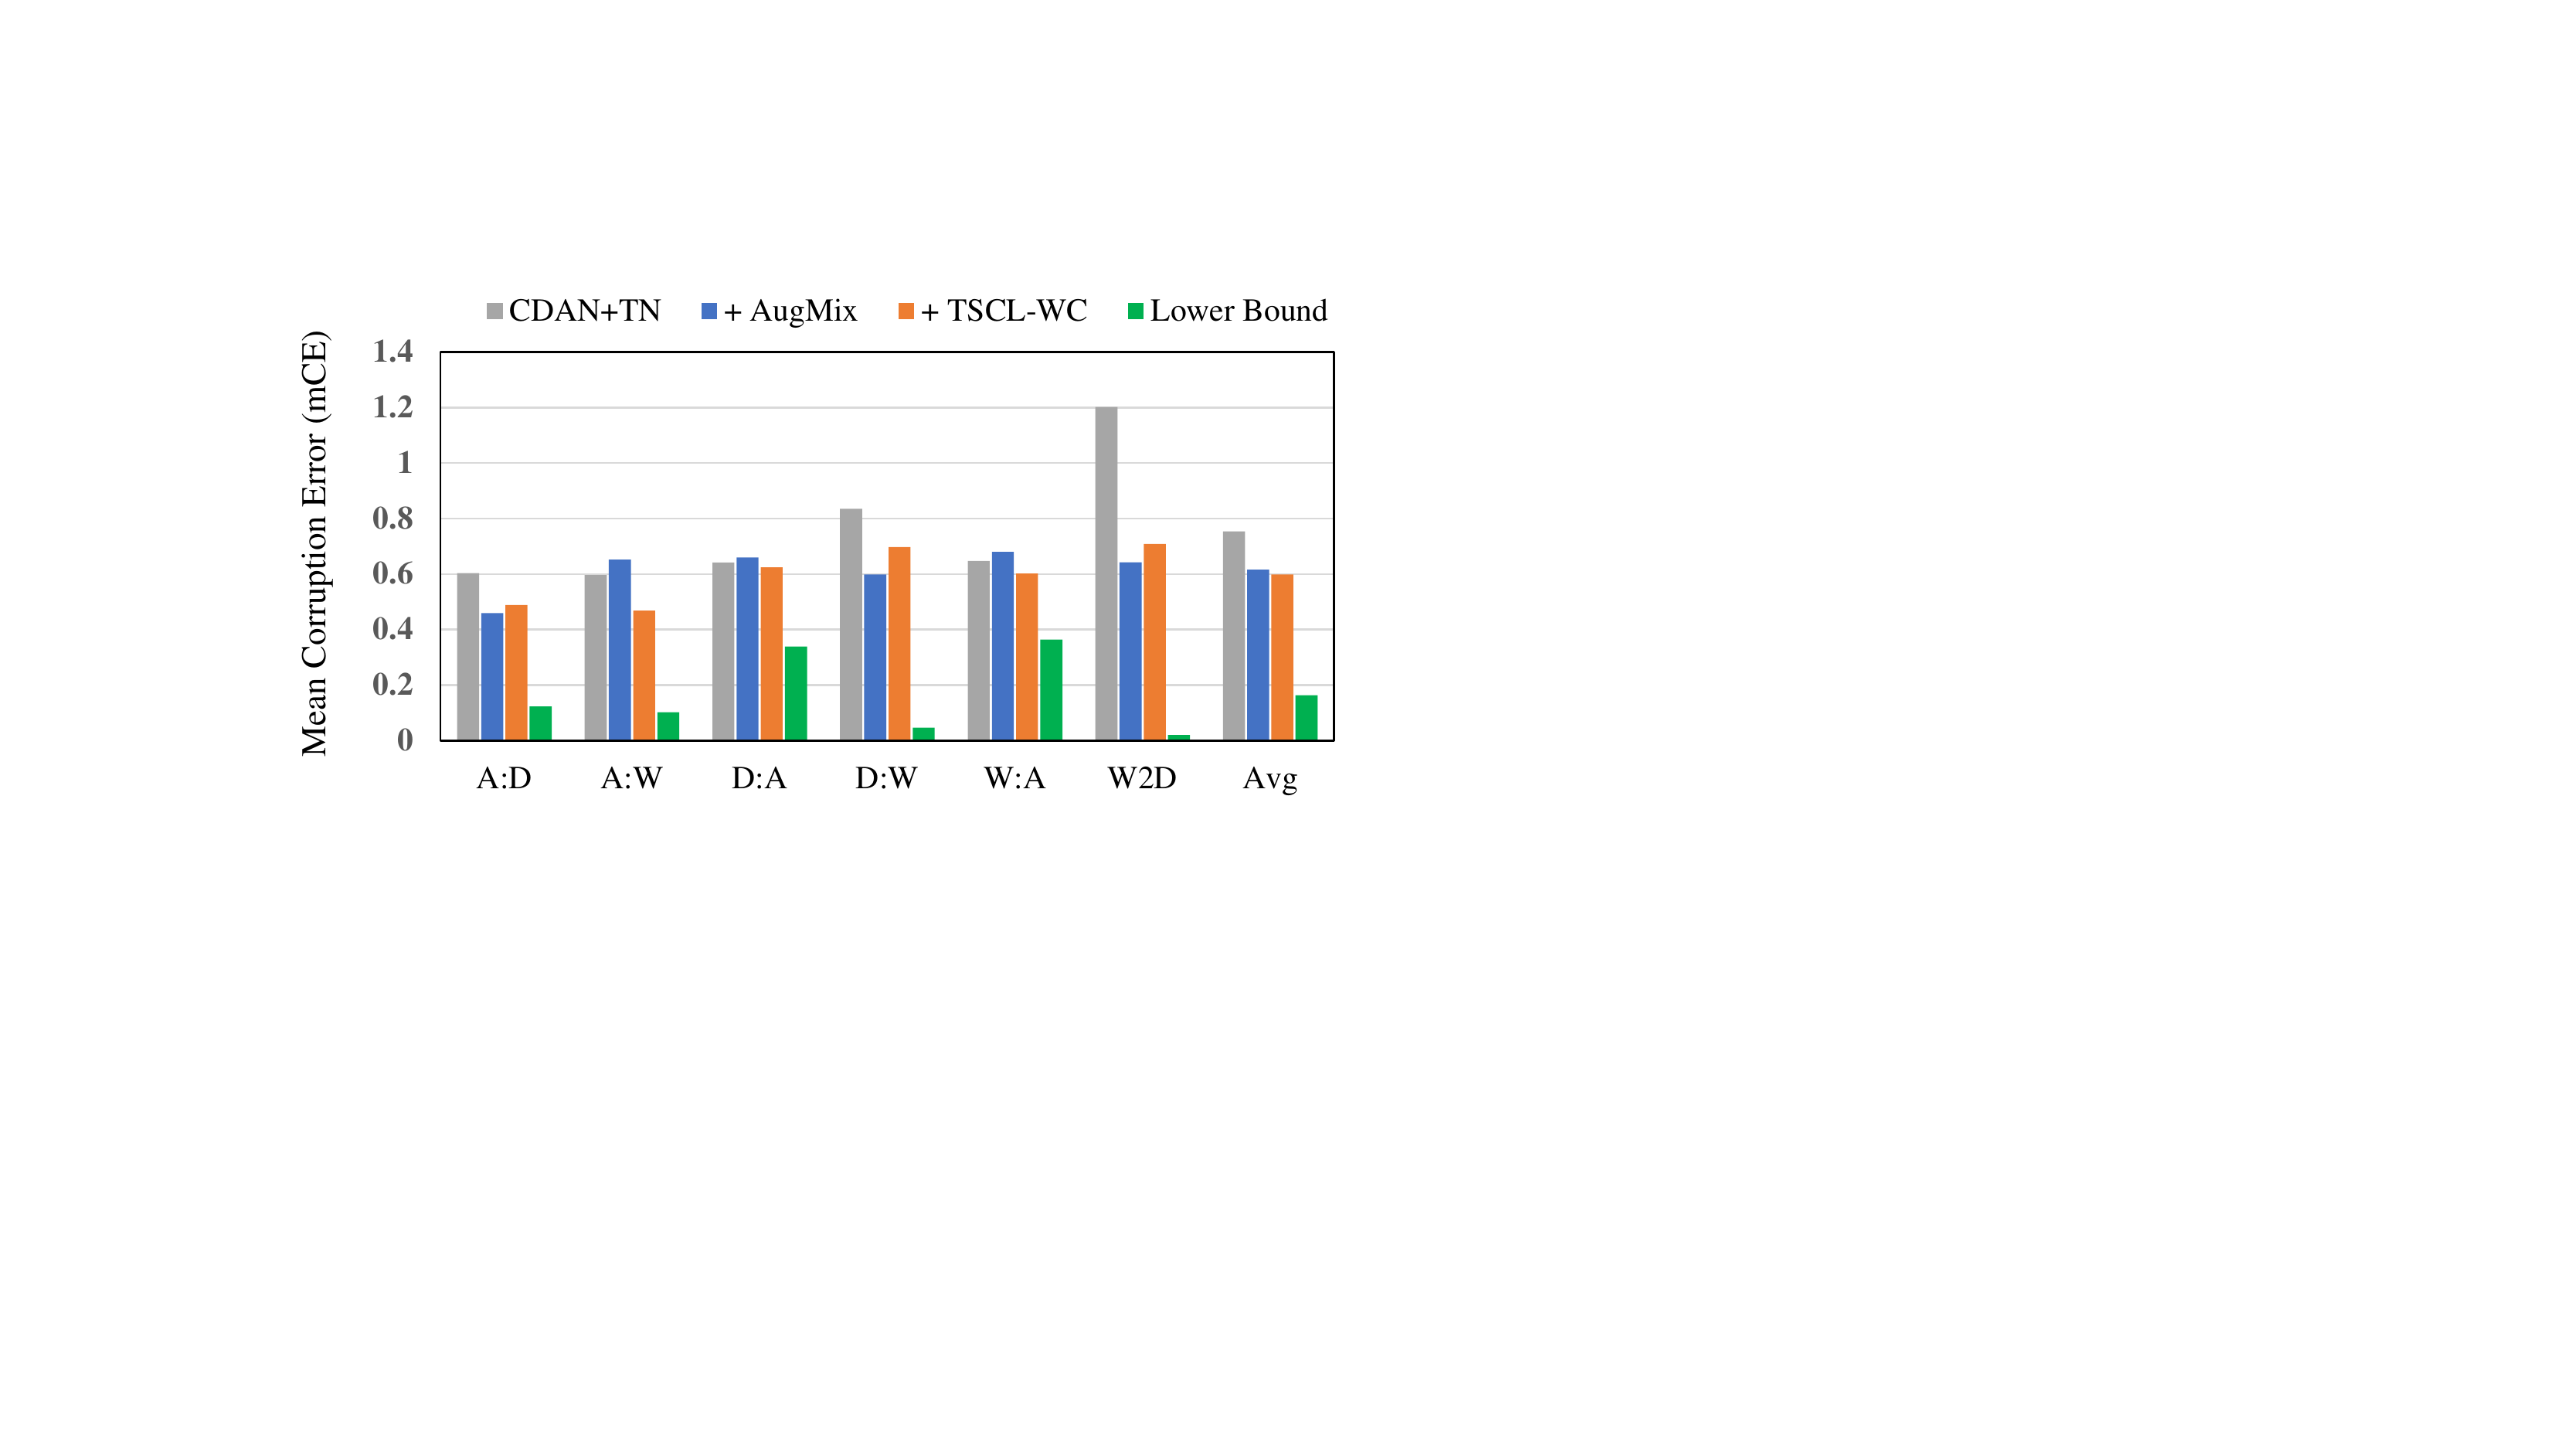}
    \caption{mCE ($\%$) on all cross-domain settings of Office-31 under CRDA (ResNet-50).}
    \label{fig:mCE-office-sup}
\end{figure}
