# Supplementary material for: Towards Corruption-Agnostic Robust Domain Adaptation
Source: arXiv:2104.10376 source file (2021-04-21)
Supplement: Supplementary file 12 [file mCE_precise-sup.tex]

\begin{figure}[!h]
    \centering
    \includegraphics[width=0.6\linewidth]{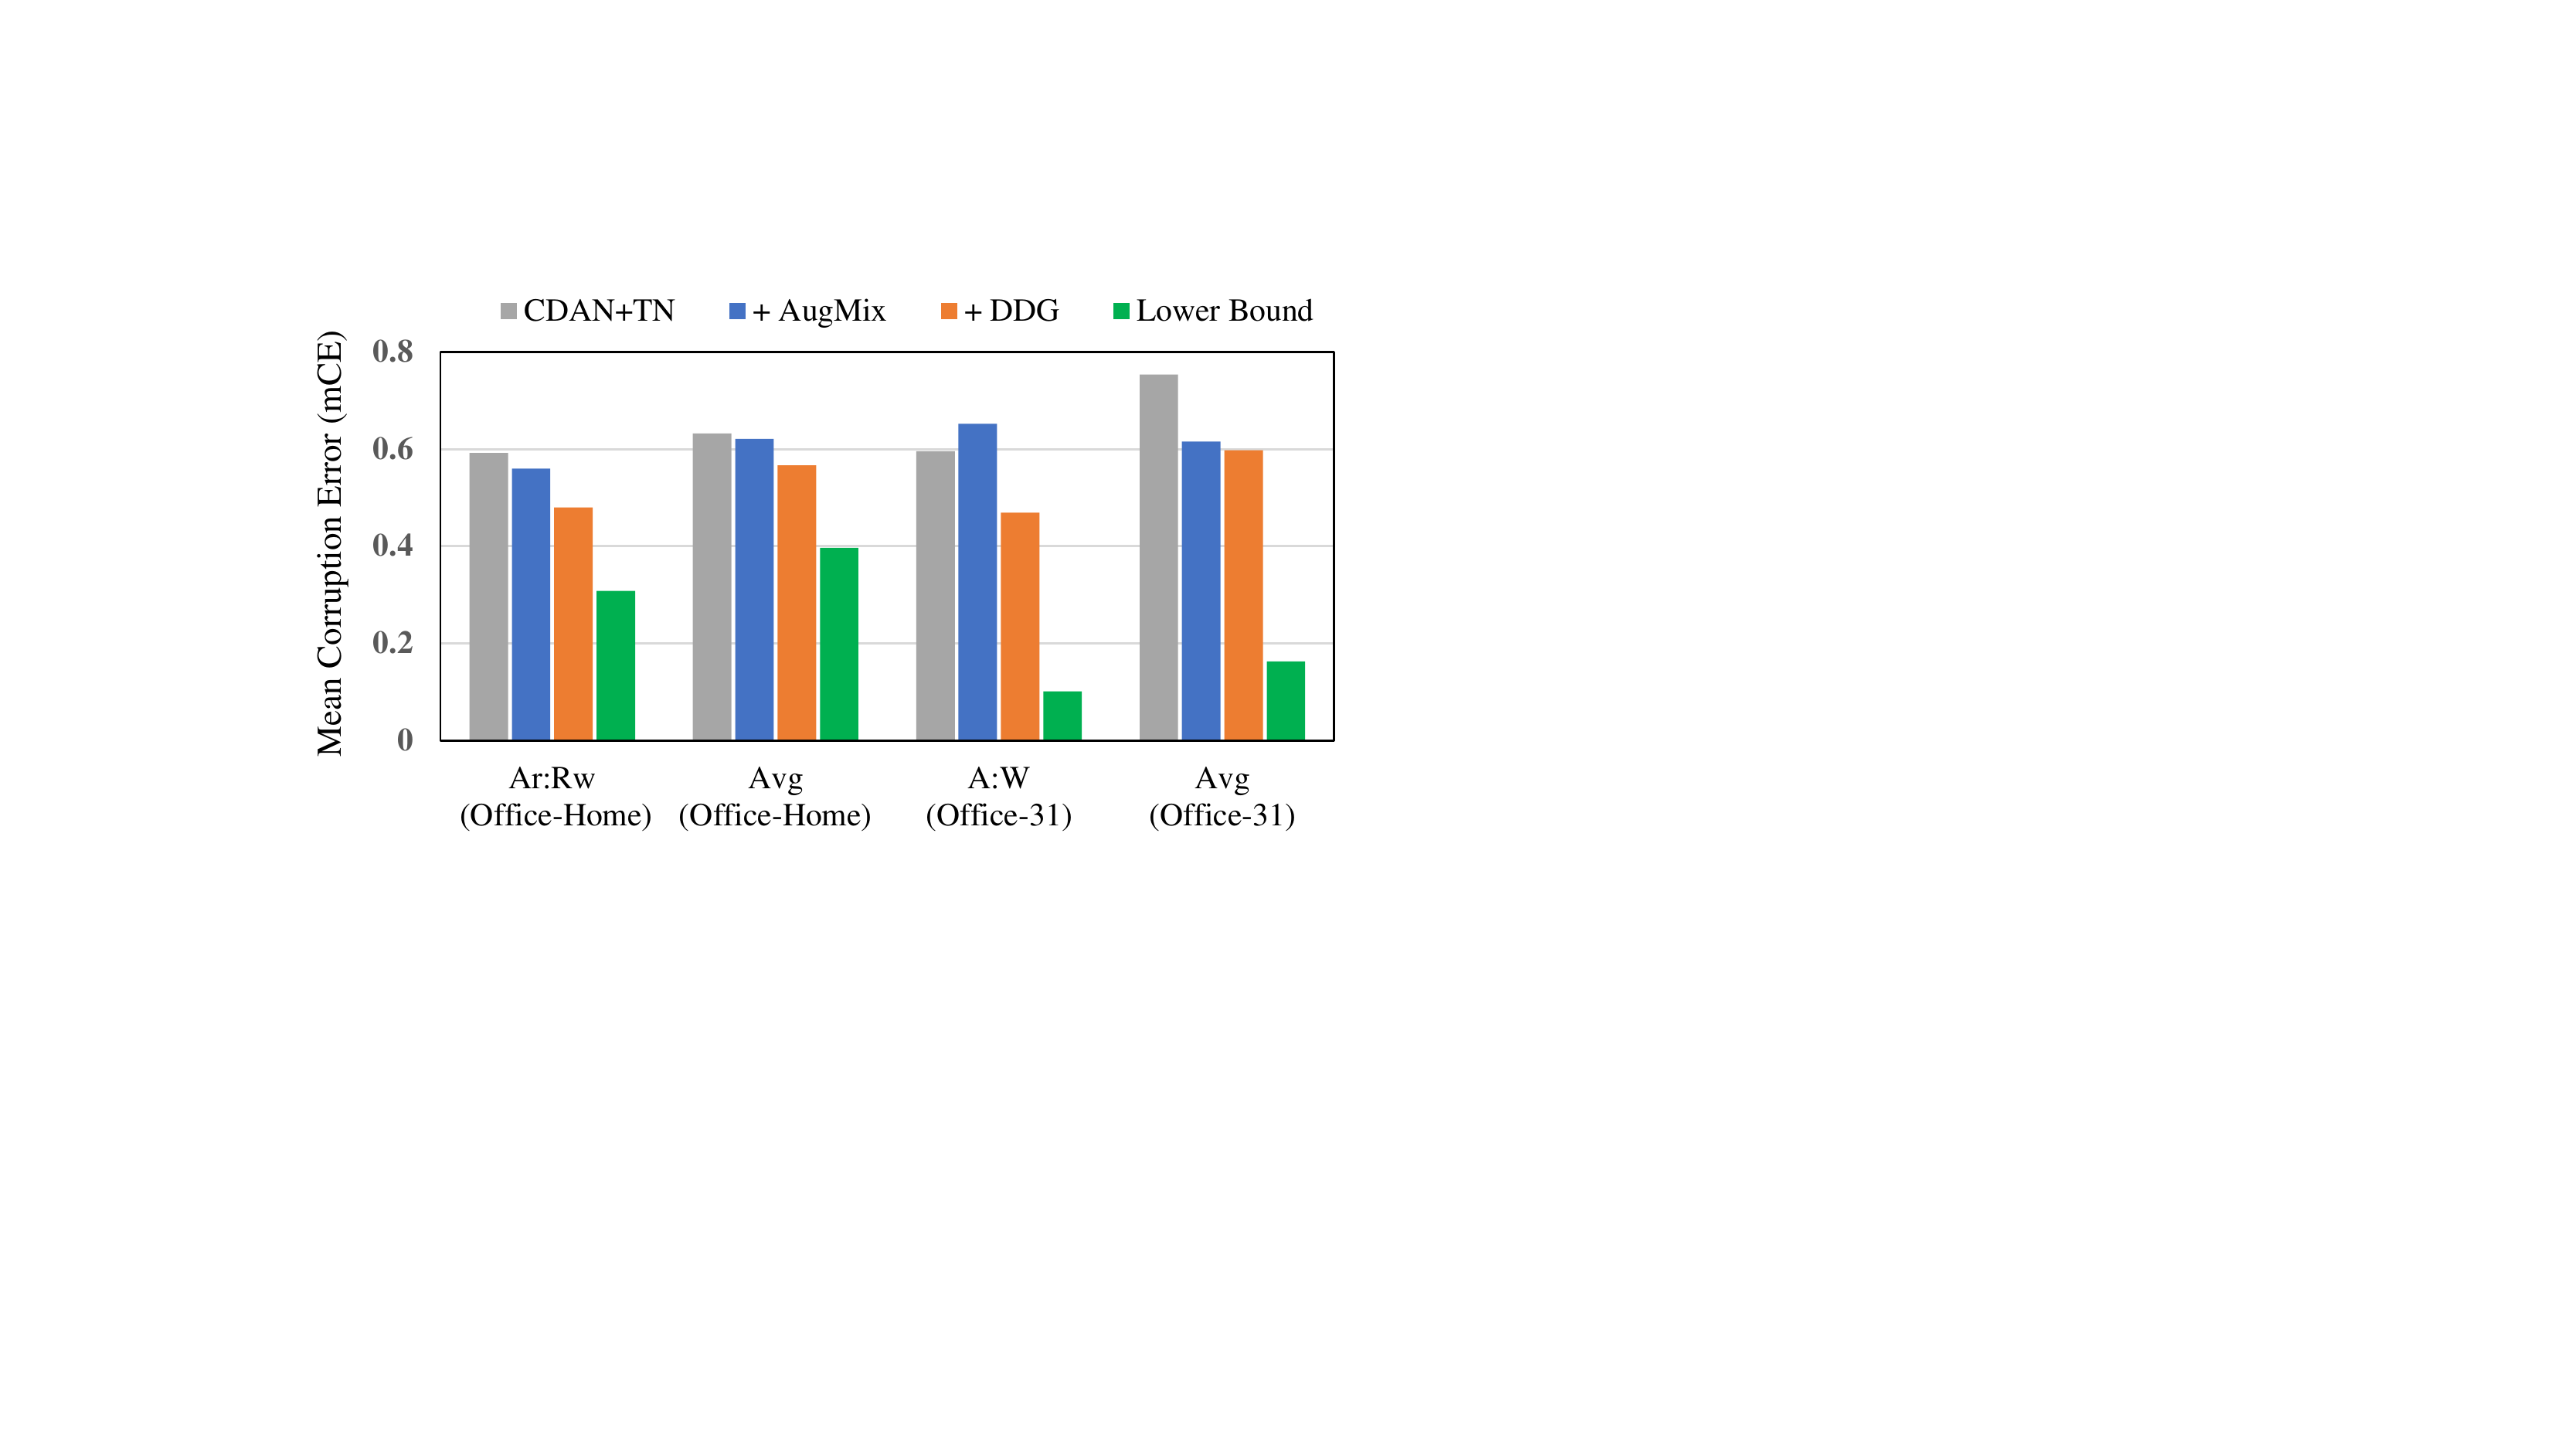}
    \caption{mCE ($\%$) on Office-Home and Office-31 datasets.}
    \label{fig:mCE-precise-sup}
\end{figure}
