# Supplementary material for: Towards Corruption-Agnostic Robust Domain Adaptation
Source: arXiv:2104.10376 source file (2021-04-21)
Supplement: Supplementary file 13 [file shift_6severity.tex]

\begin{figure}[t]
    \centering
    \includegraphics[width=0.45\textwidth]{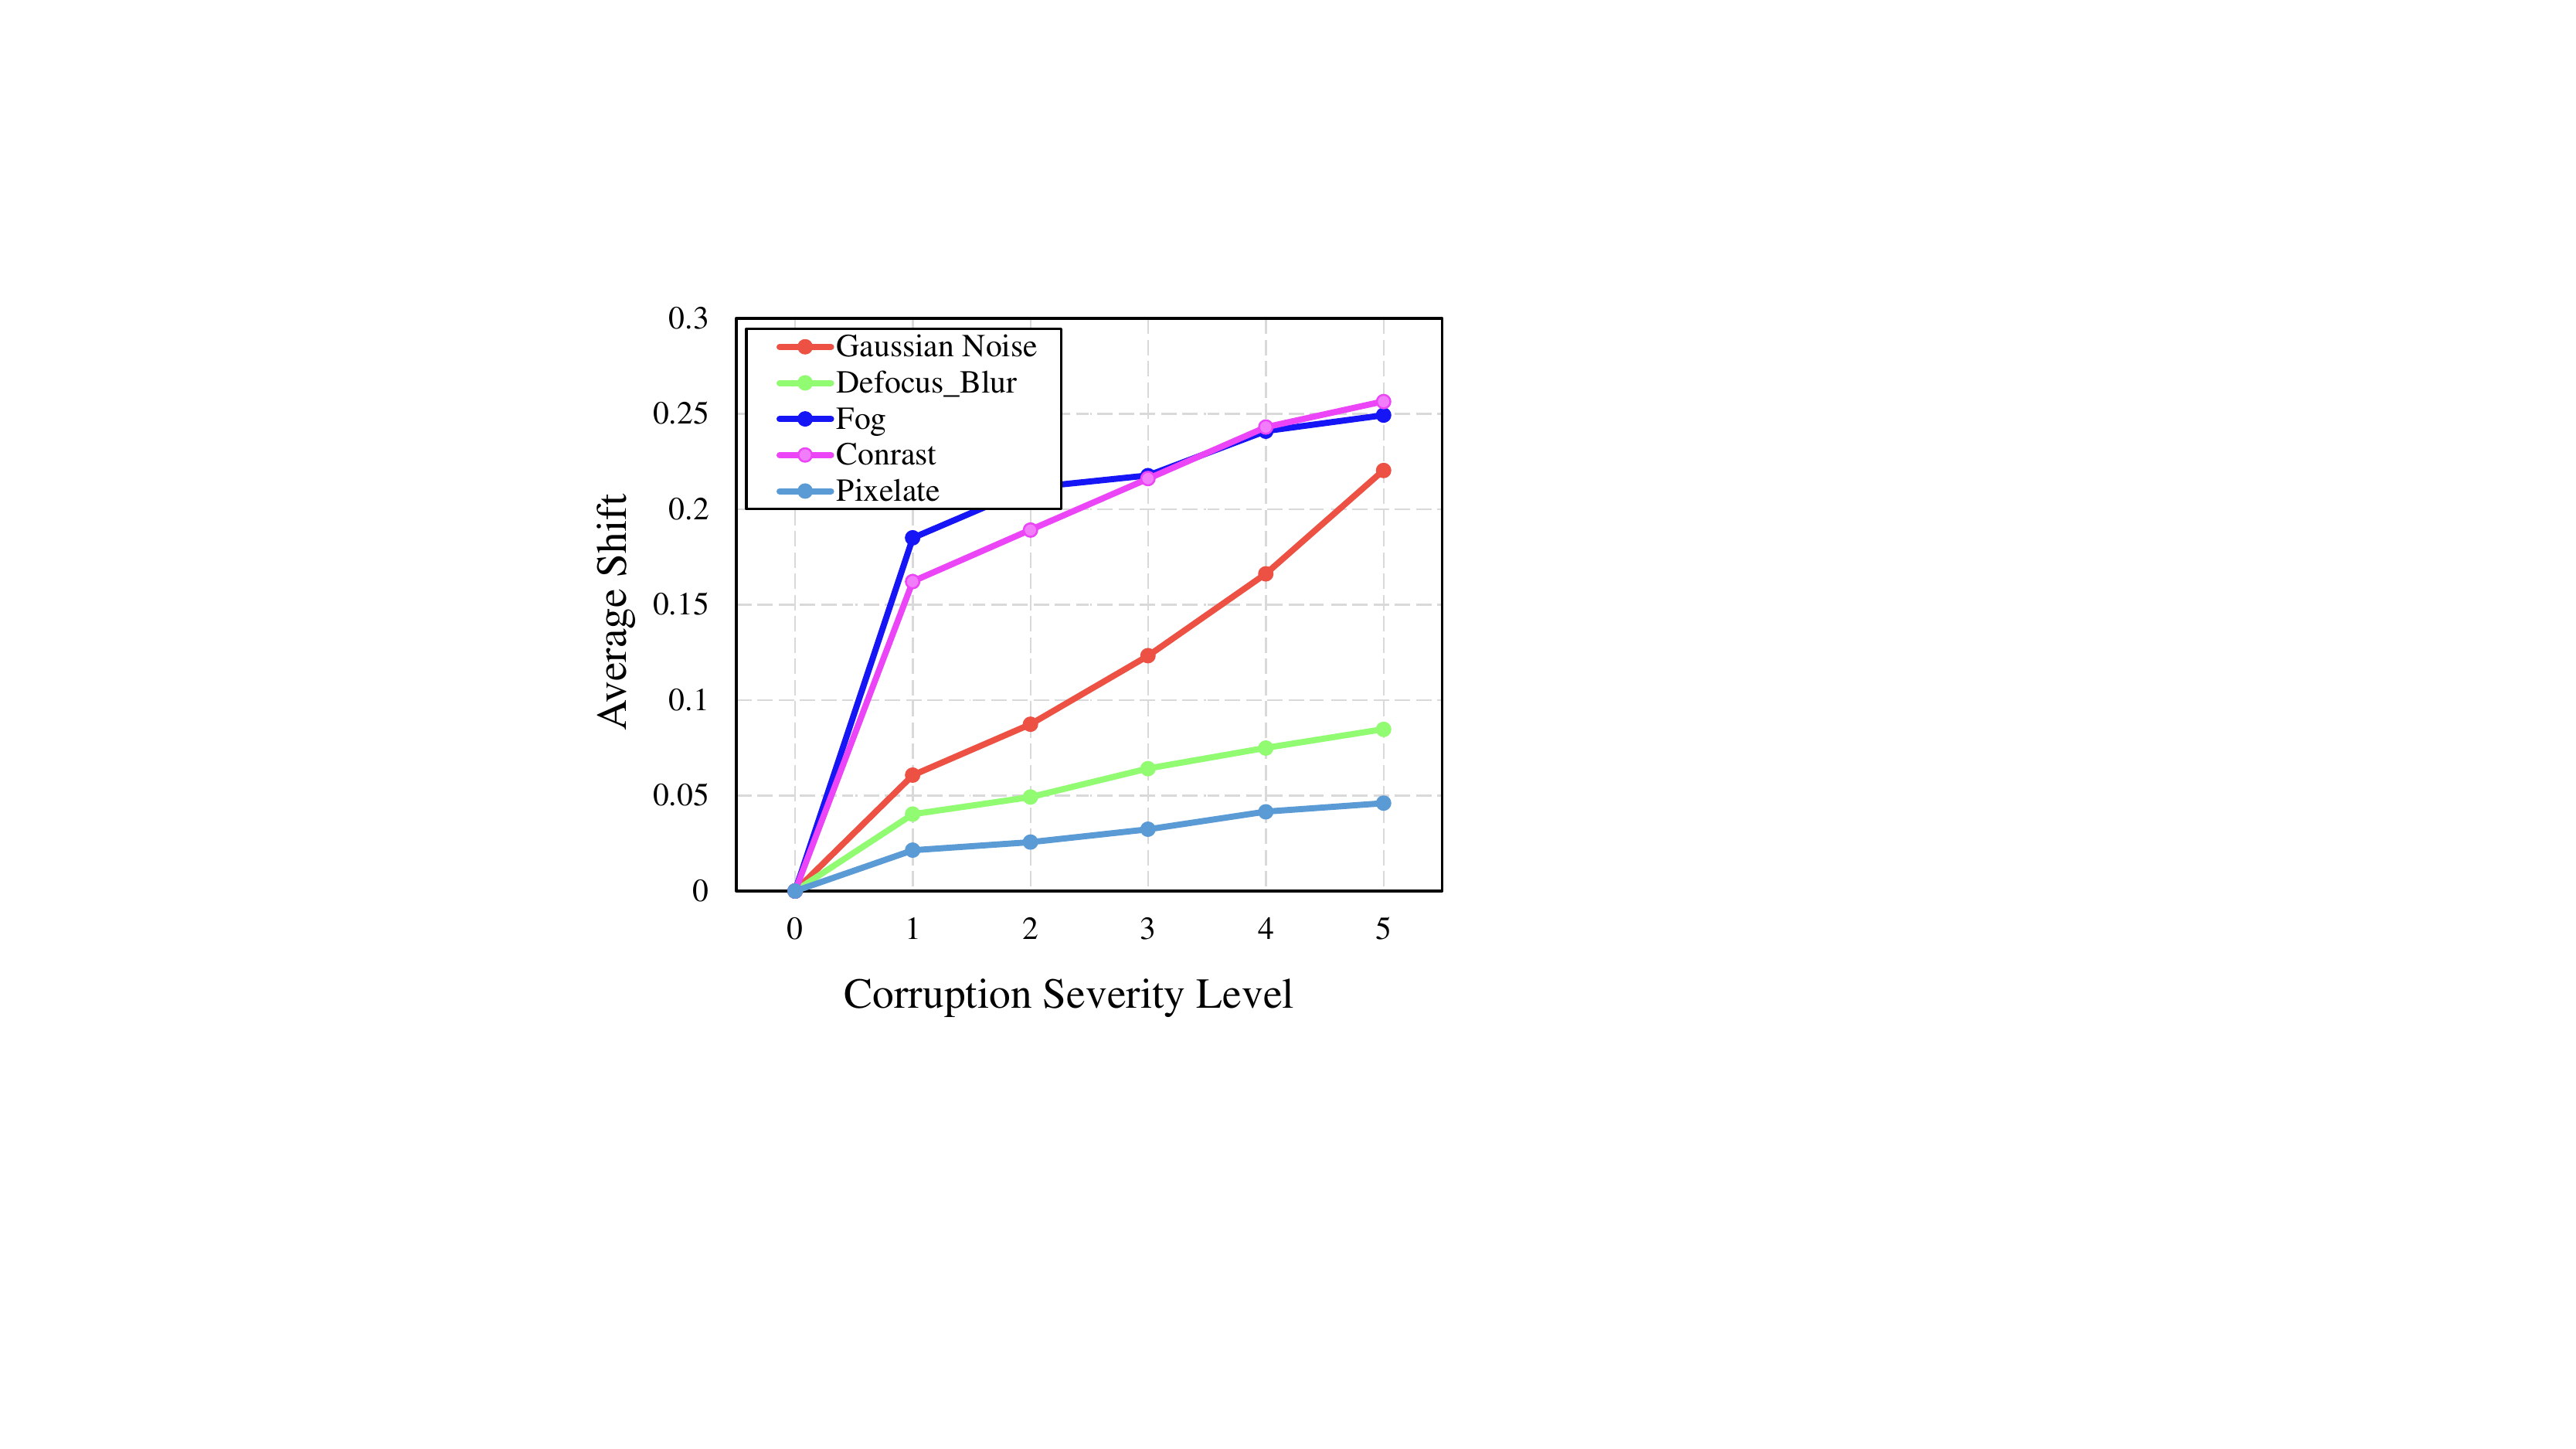}
    \caption{Average Shift of different corruptions with $6$ severity levels.}
    \label{fig:shift-6severity}
\end{figure}
