# Supplementary material for: Towards Corruption-Agnostic Robust Domain Adaptation
Source: arXiv:2104.10376 source file (2021-04-21)
Supplement: Supplementary file 17 [file Supplementary_Outline.tex]

Supplementary Material 内容
1.	15 种corruptions 的图示和描述 y
2.	3个Assumption的可靠性说明 y
3.	公式（6）的推导 y
4.	完整的TSCL结果 y
5.	AugMix的Implement Detail  x
6.	Lower bound 的具体求法，实现细节 x
8.	5.4节Order-invariant representations of corruptions的训练细节 y
9.	Training Loss的曲线 x
10.	Ablation：
    a)	超参数的影响 y
11.	解释性实验
    a)	展示并分析worst-corruption sample的图像 y
    b)	之前方法简单结合没处理好trade-off的量化指标证明
12.	为什么要选AugMix作为baseline对比 x
13. 之前基于特征的AdvTL-feature的尝试：结果及原因分析 x
14. 对于一些没有直接定义Transfer Loss 的DA x 模型，一种替代方法：训练一个鉴别器来生成Transfer Loss
    a)  出发点
    b)  方法描述
    b)  结果展示
15. AlexNet 的error rate结果 (计算mCE时用的) x
16. 其他DA模型的鲁棒性测试，说明DCAN鲁棒性相对好只是个例 x
17. 说明表3中的CLean的结果是所有鲁棒性的实验取的平均值 y
