# Supplementary material for: Towards Corruption-Agnostic Robust Domain Adaptation
Source: arXiv:2104.10376 source file (2021-04-21)
Supplement: Supplementary file 25 [file Worst-Corruption_Sample.tex]

\section{Instance of worst-corruption sample}
\label{sec:wc_sample}
% \input{latex/Supplementary_Section/imgs/wc_sample}
We show several examples of worse-corruption sample generated by our method, as well as its corresponding clean image, in Figure \ref{fig:wc_sample}.
