# Supplementary material for: Towards Corruption-Agnostic Robust Domain Adaptation
Source: arXiv:2104.10376 source file (2021-04-21)
Supplement: Supplementary file 26 [file wc_sample.tex]

\begin{figure*}[t]
    \centering
    \includegraphics[width=0.88\textwidth]{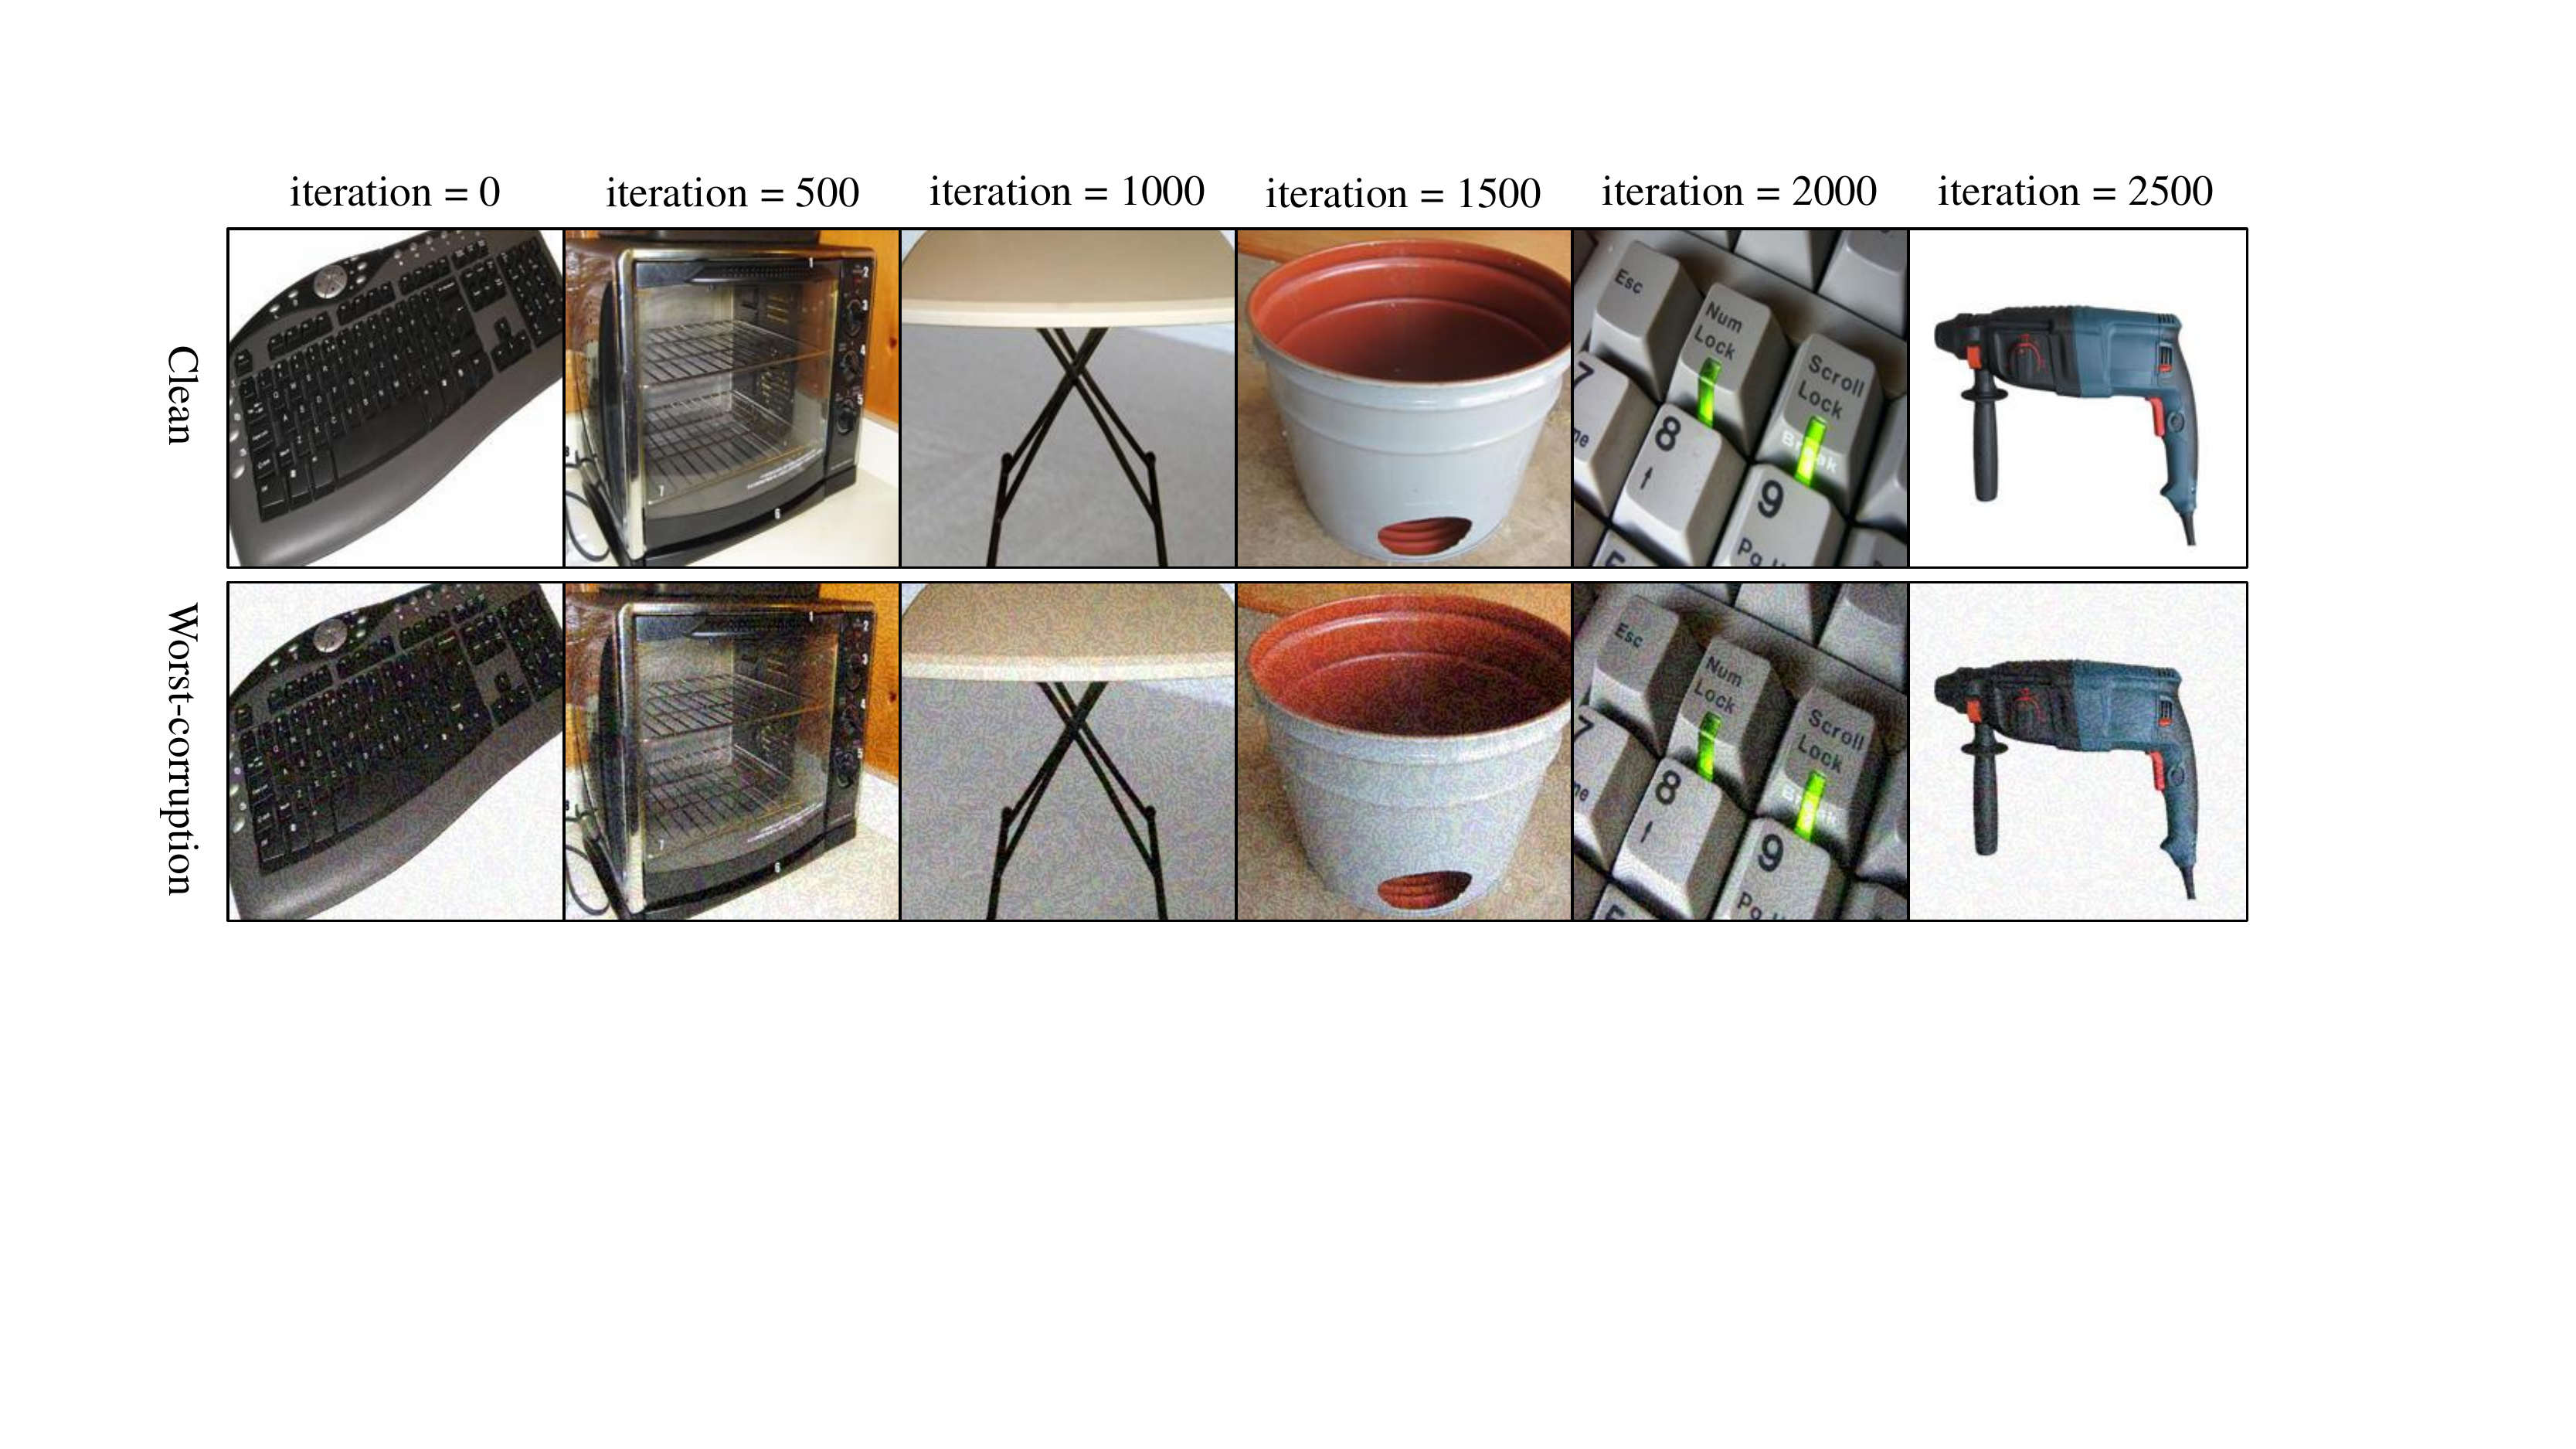}
    \caption{Worst-corruption samples of different iterations.}
    \label{fig:wc_sample}
\end{figure*}
